# Supplementary material for: Local policy search with Bayesian optimization
Source: arXiv:2106.11899 source file (2021-11-22)
Supplement: Supplementary file 1 [file Welford.tex]

\subsection{Welford's Online Algorithm}\label{appendix:welfords_online}
Welford's online algorithm \citep{Welford1962, Donald1998} is an online update of mean and variance of a vector $x \in \mathbb{R}^p$. It is especially useful for tasks where each value $x_n$ is inspected only once, because it exploits a numerically stable recurrence relation for the required statistics.
The following formulas define the recurrence relation of the sample mean $\overline{x}_n \in \mathbb{R}^p$, the squared distance from the mean $S_n\in \mathbb{R}^p$ and the unbiased sample variance $s^2_n \in \mathbb{R}^p$, each of $n$ samples.
\begin{align*}
\overline{x}_n &= \overline{x}_{n-1} + \frac{x_n - \overline{x}_{n-1}}{n}, \\
S_n &= S_{n-1} + (x_n - \overline{x}_{n-1})(x_n - \overline{x}_n), \\
s_n^2 &= \frac{S_n}{n-1}.
\end{align*}
The resulting algorithm can be split unto an update- and finalize-function as shown in the following Algorithm.
\begin{algorithm}[H]
    \caption{Welford's Online Algorithm}
    \label{algo:welfords_online}
    \begin{algorithmic}[1] % The number tells where the line numbering should start
    \State $M_0 := x_0$ \Comment{Sample mean.}
    \State $S_0 := 0$ \Comment{Squared distance from mean.}
    \State $n := 0$ \Comment{Counter.}
    \Function{Update}{$x_n$, $M_{n-1}$, $S_{n-1}$}
    	\State $n \leftarrow n+1$
    	\State $M_n = M_{n-1} + \frac{(x_n - M_{n-1})}{n}$
    	\State $S_n = S_{n-1} + (x_n - M_{n-1})(x_n - M_n)$
        \State \textbf{return} ($n$, $M_n$, $S_n$)
    \EndFunction
    \Function{Finalize}{$n$, $M_n$, $S_n$} \Comment{Compute sample variance of $n$ samples.}
    	\State $s_n^2 = \frac{S_n}{n-1}$
    	\State \textbf{return} ($M_n$, $s_n^2$)
    \EndFunction
    \end{algorithmic}
\end{algorithm}
