# Supplementary material for: Local policy search with Bayesian optimization
Source: arXiv:2106.11899 source file (2021-11-22)
Supplement: Supplementary file 2 [file result_tables.tex]

% \begin{table}[tb]
%     \centering
%     \caption{A comparison of GIBO, ARS, NG, and TRPO on the MuJoCo locomotion tasks. For each task we
% show the average number of episodes required to achieve a prescribed reward threshold, averaged
% over three random seeds. Values for the reinforcement benchmarks are taken from \citep{Recht2018}.}
%     \begin{tabular}{l l r r r r r}
%         & & \multicolumn{5}{c}{Average $\#$ episodes to reach reward threshold}\\ 
%         \toprule
%         Task & Threshold & GIBO & ARS & NG-lin & NG-rbf & TRPO-nn \\
%         \midrule 
%         Swimmer-v1 & 325 & 536 & N/A \tablefootnote{N/A means that the method did not reach the reward threshold.} & 1450 & 1550 & N/A \\ \addlinespace
%         Hopper-v1 & 3120 & 5060 & N/A & 13920 & 8640 & 10000\\ \addlinespace
% \end{tabular}
% \end{table}

% \begin{table}[tb]
%     \centering
%     \caption{A comparison of several policy search algorithms methods on the MuJoCo locomotion tasks. For each task we show the average number of timesteps required to reach a prescribed reward threshold, averaged over three random seeds. Values for the reinforcement benchmarks are taken from \citep{Recht2018}.}
%     \begin{tabular}{l l r r r r }
%         & & \multicolumn{4}{c}{Average $\#$ timesteps to hit threshold}\\ 
%         \toprule
%         Task & Threshold & GIBO & ARS & ES & TRPO \\
%         \midrule 
%         Swimmer-v1 & 128.25 & $2.21 \cdot 10^5$ & $3.54 \cdot 10^5$ & $1.39 \cdot 10^6$ & $4.59 \cdot 10^6$ \\ \addlinespace
%         Hopper-v1 & 3402.46 & N/A & N/A & $3.16 \cdot 10^7$ & $4.56 \cdot 10^6$\\ \addlinespace
% \end{tabular}
% \end{table}

% \begin{table}[tb]
%     \centering
%     \caption{A comparison of several policy search algorithms on the MuJoCo locomotion tasks. For each task we show the maximum rewards achieved after a prescribed number of simulator timesteps have been used, averaged over three random seeds. Values for the reinforcement benchmarks are taken from \citep{Recht2018}.}
%     \begin{tabular}{l l r r r r r r}
%         & & \multicolumn{6}{c}{Maximum average reward after $\#$ timesteps}\\ 
%         \toprule
%         Task & $\#$ timesteps & GIBO & ARS & PPO & A2C & CEM & TRPO \\
%         \midrule 
%         Swimmer-v1 & $10^6$ & $315$ & $ 285$ & $\approx 110$ & $\approx 30$ & $\approx 0$ & $\approx 120$ \\ \addlinespace
%         Hopper-v1 & $10^6$ & $2411$ & $2519$  & $\approx 2300$ & $\approx 900$ & $\approx 500$ & $\approx 2000$ \\ \addlinespace
% \end{tabular}
% \end{table}

% \begin{table}[tb]
%     \centering
%     \caption{A comparison of several policy search algorithms on the MuJoCo locomotion tasks. For each task we show the maximum rewards achieved after a prescribed number of simulator timesteps have been used. The values for GIBO and ARS were averaged over three random seeds. Values for the reinforcement benchmarks are taken from \citep{Recht2018}.}
%     \begin{tabular}{l l r r r r r r}
%         & & \multicolumn{6}{c}{Maximum average reward after $\#$ timesteps}\\ 
%         \toprule
%         Task & $\#$ timesteps & GIBO & ARS & PPO & A2C & CEM & TRPO \\
%         \midrule 
%         Hopper-v1 & $2 \cdot 10^6$ & $2557$ & $2707$ & $\approx 3000$ & $\approx 1100$ & $\approx 1500$ & $\approx 1250$ \\ \addlinespace
% \end{tabular}
% \end{table}
