# Supplementary material for: Local policy search with Bayesian optimization
Source: arXiv:2106.11899 source file (2021-11-22)
Supplement: Supplementary file 3 [file neurips_checklist.tex]

\pagebreak
\section*{Checklist}

\begin{enumerate}

\item For all authors...
\begin{enumerate}
  \item Do the main claims made in the abstract and introduction accurately reflect the paper's contributions and scope?
    \answerYes{}
  \item Did you describe the limitations of your work?
    \answerYes{} We point out during the paper and especially in the conclusion \sect\ref{sec:conclusion} that the performance of GIBO hinges on prior knowledge of the objective function in the form of GP hyperparamters.
  \item Did you discuss any potential negative societal impacts of your work?
    \answerYes{} Our work doesn't describe a specific application, but a general optimization algorithm. We shortly discuss automated decision making in the conclusion \sect\ref{sec:conclusion}. 
  \item Have you read the ethics review guidelines and ensured that your paper conforms to them?
    \answerYes{}
\end{enumerate}

\item If you are including theoretical results...
\begin{enumerate}
  \item Did you state the full set of assumptions of all theoretical results?
    \answerNA{}
	\item Did you include complete proofs of all theoretical results?
    \answerNA{}
\end{enumerate}

\item If you ran experiments...
\begin{enumerate}
  \item Did you include the code, data, and instructions needed to reproduce the main experimental results (either in the supplemental material or as a URL)?
    \answerYes{} \url{https://github.com/gibo-neurips-2021/GIBO.git}
  \item Did you specify all the training details (e.g., data splits, hyperparameters, how they were chosen)?
    \answerYes{} See Appendix \ref{appendix:hyperparameters}.
	\item Did you report error bars (e.g., with respect to the random seed after running experiments multiple times)?
    \answerYes{} See \sect\ref{sec:results} for the variance after 300 query points.
    We choose not to plot error bars in the learning curves for readability reasons. Since the results are plotted on a log scale the error bars are hard to read.
	\item Did you include the total amount of compute and the type of resources used (e.g., type of GPUs, internal cluster, or cloud provider)?
    \answerNo{} We used a virtual machine (VM) of an internal VM cluster, 16 GB RAM, 8 VCPUs, total disk 160 GB, no GPU.
\end{enumerate}

\item If you are using existing assets (e.g., code, data, models) or curating/releasing new assets...
\begin{enumerate}
  \item If your work uses existing assets, did you cite the creators? 
    \answerYes{}
    We use the OpenAI Gym environments as well as the MuJoCo engine.
  \item Did you mention the license of the assets?
    \answerYes{}
    See Appendix~\ref{appendix:implementation}. 
  \item Did you include any new assets either in the supplemental material or as a URL?
    \answerNA{}{}
  \item Did you discuss whether and how consent was obtained from people whose data you're using/curating?
    \answerNA{}
  \item Did you discuss whether the data you are using/curating contains personally identifiable information or offensive content?
    \answerNA{}
\end{enumerate}

\item If you used crowdsourcing or conducted research with human subjects...
\begin{enumerate}
  \item Did you include the full text of instructions given to participants and screenshots, if applicable?
    \answerNA{}
  \item Did you describe any potential participant risks, with links to Institutional Review Board (IRB) approvals, if applicable?
    \answerNA{}
  \item Did you include the estimated hourly wage paid to participants and the total amount spent on participant compensation?
    \answerNA{}
\end{enumerate}

\end{enumerate}
\vfill
